# Supplementary material for: Real-time 3D Pose Estimation with a Monocular Camera Using Deep Learning and Object Priors On an Autonomous Racecar
Source: arXiv:1809.10548 source file (2018-09-27)
Supplement: Supplementary file 1 [file appendix.tex]

%% ----------------------------------------------------------------------------
% BIWI SA/MA thesis template
%
% Created 09/29/2006 by Andreas Ess
% Extended 13/02/2009 by Jan Lesniak - jlesniak@vision.ee.ethz.ch
%% ----------------------------------------------------------------------------
\chapter{The First Appendix}

In the appendix, list the following material: 

\begin{itemize}
 \item Data (evaluation tables, graphs etc.)
 \item Program code
 \item Further material 
\end{itemize}
